# Supplementary material for: Tri-Modal Motion Retrieval by Learning a Joint Embedding Space
Source: arXiv:2403.00691 source file (2024-03-01)
Supplement: Supplementary file 1 [file X_suppl.tex]

\clearpage
\setcounter{page}{1}
\maketitlesupplementary

\section{Rendering RGB Videos for KIT-ML Dataset and HumanML3D Dataset}
AMASS~\cite{mahmood2019amass} dataset only contains motion capture data without any RGB videos. In this regard, for each motion capture sequence, an avatar is randomly picked from 13 different avatars shown in Figure~\ref{fig:amass_avatars}, animated and rendered to form its corresponding RGB videos of size $512\times 512$, obtained using one of the 4 predefined lightning conditions displayed in Table~\ref{tab:light}. These 4 lightning conditions represent the positions of top center, left and right top, left and right bottom with different strength of illumination ranging from 0 to 1. Additionally, we adjust the trajectory (global translations of each frame) of each sequence properly to avoid the rendered avatar out of the camera scope. Combining these adjusted global translations with the original SMPL pose and shape annotations, we obtain the new annotations for each sequence in AMASS. Combined with annotated text and SMPL motion, we obtain the associated RGB videos for HumanML3D and KIT datasets.

\begin{figure*}[ht]
    \centering
    \includegraphics[width=\textwidth]{Picture/amass_all_avatars.jpg}
    \caption{\textbf{Front and Back Views of 13 Avatars Used in Video Synthesis.}}
    \label{fig:amass_avatars}
\end{figure*}

\begin{table}[h!]
\centering
\small
\setlength{\tabcolsep}{0.6pt}
\begin{tabular}{c|*{1}{>{\centering\arraybackslash}m{3cm}}|*{1}{>{\centering\arraybackslash}m{3cm}}}
\midrule
\textbf{Lightning} & \multicolumn{1}{c|}{\textbf{Position}} & \multicolumn{1}{c}{\textbf{Color}} \\
\midrule
1 & \([0, 0, -300]\) & \([1.0, 1.0, 1.0]\) \\
\midrule
2 & \([-300, -300, -300]\) & \([0.8, 0.8, 0.8]\) \\
  & \([300, -300, -300]\) & \([0.8, 0.8, 0.8]\) \\
\midrule
3 & \([0, 0, -300]\) & \([1, 1, 1]\) \\
  & \([-300, 0, -300]\) & \([0.4, 0.4, 0.4]\) \\
\midrule
4 & \([300, 0, -300]\) & \([0.4, 0.4, 0.4]\) \\
  & \([-300, 0, -300]\) & \([1, 1, 1]\) \\
\bottomrule
\end{tabular}
\caption{Your caption here.}
\label{tab:light}
\end{table}
% 
% \begin{figure}[t]
%     \centering
%     \includegraphics[width=0.5\textwidth]{Picture/video_encoder.png}
%     \caption{Caption\red{may put to supplementary as this architecture is not new things.}}
%     \label{fig:1}
% \end{figure}

\section{Ablation Study}
We conduct ablation studies on four hyper-parameters: the reconstruction weight ${\lambda_{recon}}$, the negative filtering threshold $\epsilon$, the batch size $B$ and the latent dimension $C$. The purpose of the reconstruction loss is to ensure that no information is lost when translating between modalities. In our design of a custom attention mechanism, which aims to enhance alignment between the three modalities, we consider its relative weight in the overall loss to be significant. Upon testing four different values, we found that a weight of 0.1 yields the best performance. The ablation study for the reconstruction weight is shown in table~\ref{tab recon}. For the negative filtering threshold $\epsilon$, we aim to identify an optimal value that ensures the model effectively aggregates data pairs containing similar information. After testing five different values, we find that a threshold of 0.8 yields the optimal outcome. The ablation study for the negative filtering threshold is shown in table~\ref{tab threshold}. For the batch size $B$ and the latent dim $C$, we test with four commonly used values respectively, we find that the best value for the batch size and the latent dimension is 64 and 512. The ablation studies are shown in table~\ref{tab bs} and table~\ref{tab latentdim}.

\begin{table}[t]
\centering
\small
\vspace{-1mm}
\setlength{\tabcolsep}{0.6pt}
\begin{tabular}{c|*{4}{>{\centering\arraybackslash}m{0.9cm}}|*{4}{>{\centering\arraybackslash}m{0.9cm}}}
\toprule
\textbf{Re Weight} & \multicolumn{4}{c|}{\textbf{Text-motion retrieval}} & \multicolumn{4}{c}{\textbf{Video-to-motion retrieval}} \\
${\lambda_{recon}}$ & R@1↑ & R@2↑ & R@3↑ & MedR↓ & R@1↑ & R@2↑ & R@3↑ & MedR↓ \\
\midrule
0.001 & 18.11 & 25.16 & 34.30 & 13.00 & 22.41 & 31.49 & 46.53 & 10.00 \\
0.01 & 27.26 & 37.78 & \bf48.91 & 6.00 & 34.19 & 47.31 & 58.88 & 4.00 \\
0.1 & \bf30.86 & \bf41.80 & 48.63 & \bf4.00 & \bf36.91 & \bf49.80 & \bf60.94 & \bf3.00 \\
1.0 & 24.15 & 32.28 & 41.12 & 9.00 & 31.76 & 43.58 & 54.29 & 7.00 \\
\bottomrule
\end{tabular}
\vspace{-3mm}
\caption{\textbf{Ablation study for the reconstruction weight.} We test four values for the reconstruction weight, the research outcome shows that 0.1 is the most appropriate value.}
\label{tab recon}
\end{table}

\begin{table}[t]
\centering
\small
\vspace{-3mm}
\setlength{\tabcolsep}{0.6pt}
\begin{tabular}{c|*{4}{>{\centering\arraybackslash}m{0.9cm}}|*{4}{>{\centering\arraybackslash}m{0.9cm}}}
\toprule
\textbf{Threshold} & \multicolumn{4}{c|}{\textbf{Text-to-motion retrieval}} & \multicolumn{4}{c}{\textbf{Video-to-motion retrieval}} \\
$\epsilon$ & R@1↑ & R@2↑ & R@3↑ & MedR↓ & R@1↑ & R@2↑ & R@3↑ & MedR↓ \\
\midrule
0.70 & 25.90 & 37.46 & 45.79 & 5.00 & 31.21 & 45.37 & 58.44 & 5.00 \\
0.75 & 27.18 & 40.23 & 48.21 & \bf4.00 & 34.15 & 47.29 & 59.71 & 4.00 \\
0.80 & \bf30.86 & \bf41.80 & \bf48.63 & \bf4.00 & \bf36.91 & \bf49.80 & \bf60.94 & \bf3.00 \\
0.85 & 26.43 & 38.22 & 47.81 & 5.00 & 33.97 & 46.38 & 57.47 & 5.00 \\
0.90 & 22.19 & 32.33 & 41.48 & 7.00 & 29.29 & 44.62 & 58.12 & 6.00 \\
\bottomrule
\end{tabular}
\vspace{-3mm}
\caption{\textbf{ablation study for the negative filtering threshold.} We test five values for the negative filtering threshold, showing that 0.8 is the most appropriate value.}
\label{tab threshold}
\end{table}

\begin{table}[t]
\centering
\small
\vspace{-3mm}
\setlength{\tabcolsep}{0.6pt}
\begin{tabular}{c|*{4}{>{\centering\arraybackslash}m{0.9cm}}|*{4}{>{\centering\arraybackslash}m{0.9cm}}}
\toprule
\textbf{Batch size} & \multicolumn{4}{c|}{\textbf{Text-to-motion retrieval}} & \multicolumn{4}{c}{\textbf{Video-to-motion retrieval}} \\
{$B$} & R@1↑ & R@2↑ & R@3↑ & MedR↓ & R@1↑ & R@2↑ & R@3↑ & MedR↓ \\
\midrule
16 & 25.12 & 37.69 & 46.18 & 6.00 & 31.35 & 45.77 & 55.36 & 6.00 \\
32 & 29.17 & 41.55 & \bf48.98 & \bf4.00 & 36.77 & \bf49.96 & 60.74 & \bf3.00 \\
64 & \bf30.86 & \bf41.80 & 48.63 & \bf4.00 & \bf36.91 & 49.80 & \bf60.94 & \bf3.00 \\
128 & 27.35 & 39.29 & 47.38 & 5.00 & 34.98 & 48.58 & 59.58 & 4.00 \\
\bottomrule
\end{tabular}
\vspace{-3mm}
\caption{\textbf{ablation study for the batch size.} We test four values for the batch size, showing that 64 is the most appropriate value.}
\label{tab bs}
\end{table}

\begin{table}[t]
\centering
\small
\vspace{-3mm}
\setlength{\tabcolsep}{0.6pt}
\begin{tabular}{c|*{4}{>{\centering\arraybackslash}m{0.9cm}}|*{4}{>{\centering\arraybackslash}m{0.9cm}}}
\toprule
\textbf{Latent dim} & \multicolumn{4}{c|}{\textbf{Text-to-motion retrieval}} & \multicolumn{4}{c}{\textbf{Video-to-motion retrieval}} \\
$C$ & R@1↑ & R@2↑ & R@3↑ & MedR↓ & R@1↑ & R@2↑ & R@3↑ & MedR↓ \\
\midrule
128 & 24.68 & 38.94 & 45.53 & 6.00 & 31.13 & 46.25 & 58.97 & 5.00 \\
256 & 29.71 & 41.34 & 47.95 & \bf4.00 & 34.38 & 47.83 & 59.72 & 4.00 \\
512 & \bf30.86 & \bf41.80 & \bf48.63 & \bf4.00 & \bf36.91 & \bf49.80 & \bf60.94 & \bf3.00 \\
1024 & 29.18 & 40.94 & 48.21 & 4.00 & 33.96 & 48.33 & 59.49 & 4.00 \\
\bottomrule
\end{tabular}
\vspace{-3mm}
\caption{\textbf{ablation study for the latent dimension.} We test four values for the latent dimension, showing that 512 is the most appropriate value.}
\label{tab latentdim}
\end{table}

\section{Attention Score}
In our approach, we leverage motion as the query to extract relevant information from both text and video modalities. This strategic extraction is quantified by computing the respective weights of text, video, and motion in the final representation, found to be 0.1147, 0.2170, and 0.6684, respectively. This weighting underscores the substantial contribution of each modality to our model. Notably, as videos are rendered and animated from motion sequences, and given that text and motion often exhibit a considerable spatial distance, the weight of the video modality is higher than that of text.

\section{Additional Qualitative Results}
In Figure~\ref{fig:4}, we present additional qualitative results. For the text-to-motion retrieval task, four supplementary outcomes are included. The first row features two randomly selected text descriptions from our test dataset. These results demonstrate our model's proficiency in accurately retrieving the corresponding ground-truth motion at the top rank. In the second row, we introduce two text descriptions not found in the existing database. However, these texts contain motions like ``hop'' and ``swim'', which can be found in the database. Intriguingly, our model displays its capability to generalize by precisely retrieving motion sequences that match the actions described in these novel texts.
In the case of synthetic video-to-motion retrieval, we use four randomly chosen videos as query inputs, showcasing motions such as ``picking up'', ``running around'', ``kicking'', and ``swinging''. Impressively, for all four queries, our model identifies the correct ground-truth motion as the top result. Lastly, in the real-life video-to-motion retrieval scenario, we input four distinct videos featuring different individuals. Our model exhibits exceptional accuracy in successfully demonstrating the exact motions depicted in each video.
\begin{figure*}
    \centering
    \vspace{-9mm}
    \includegraphics[width=\textwidth]{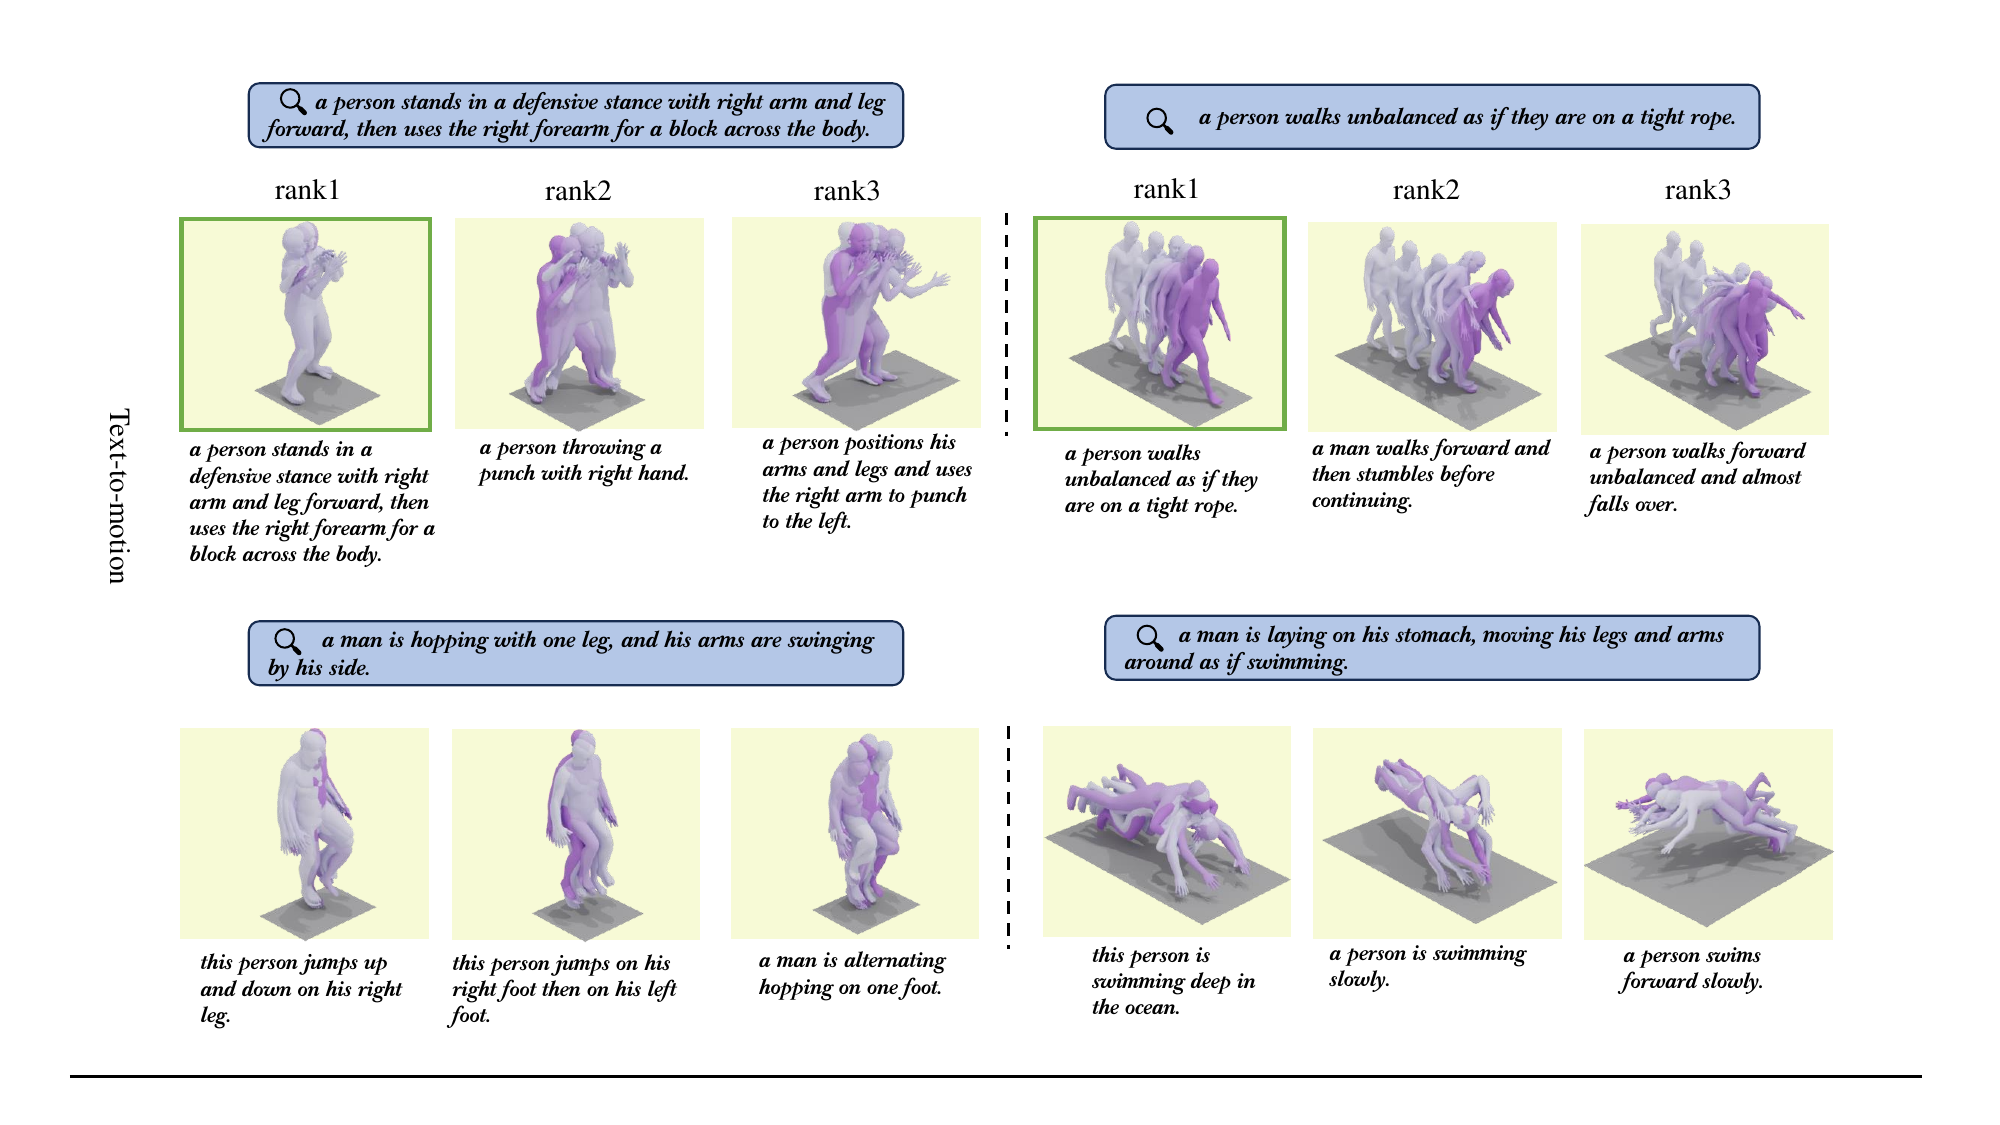}
    \vspace{-2mm}
    \includegraphics[width=\textwidth]{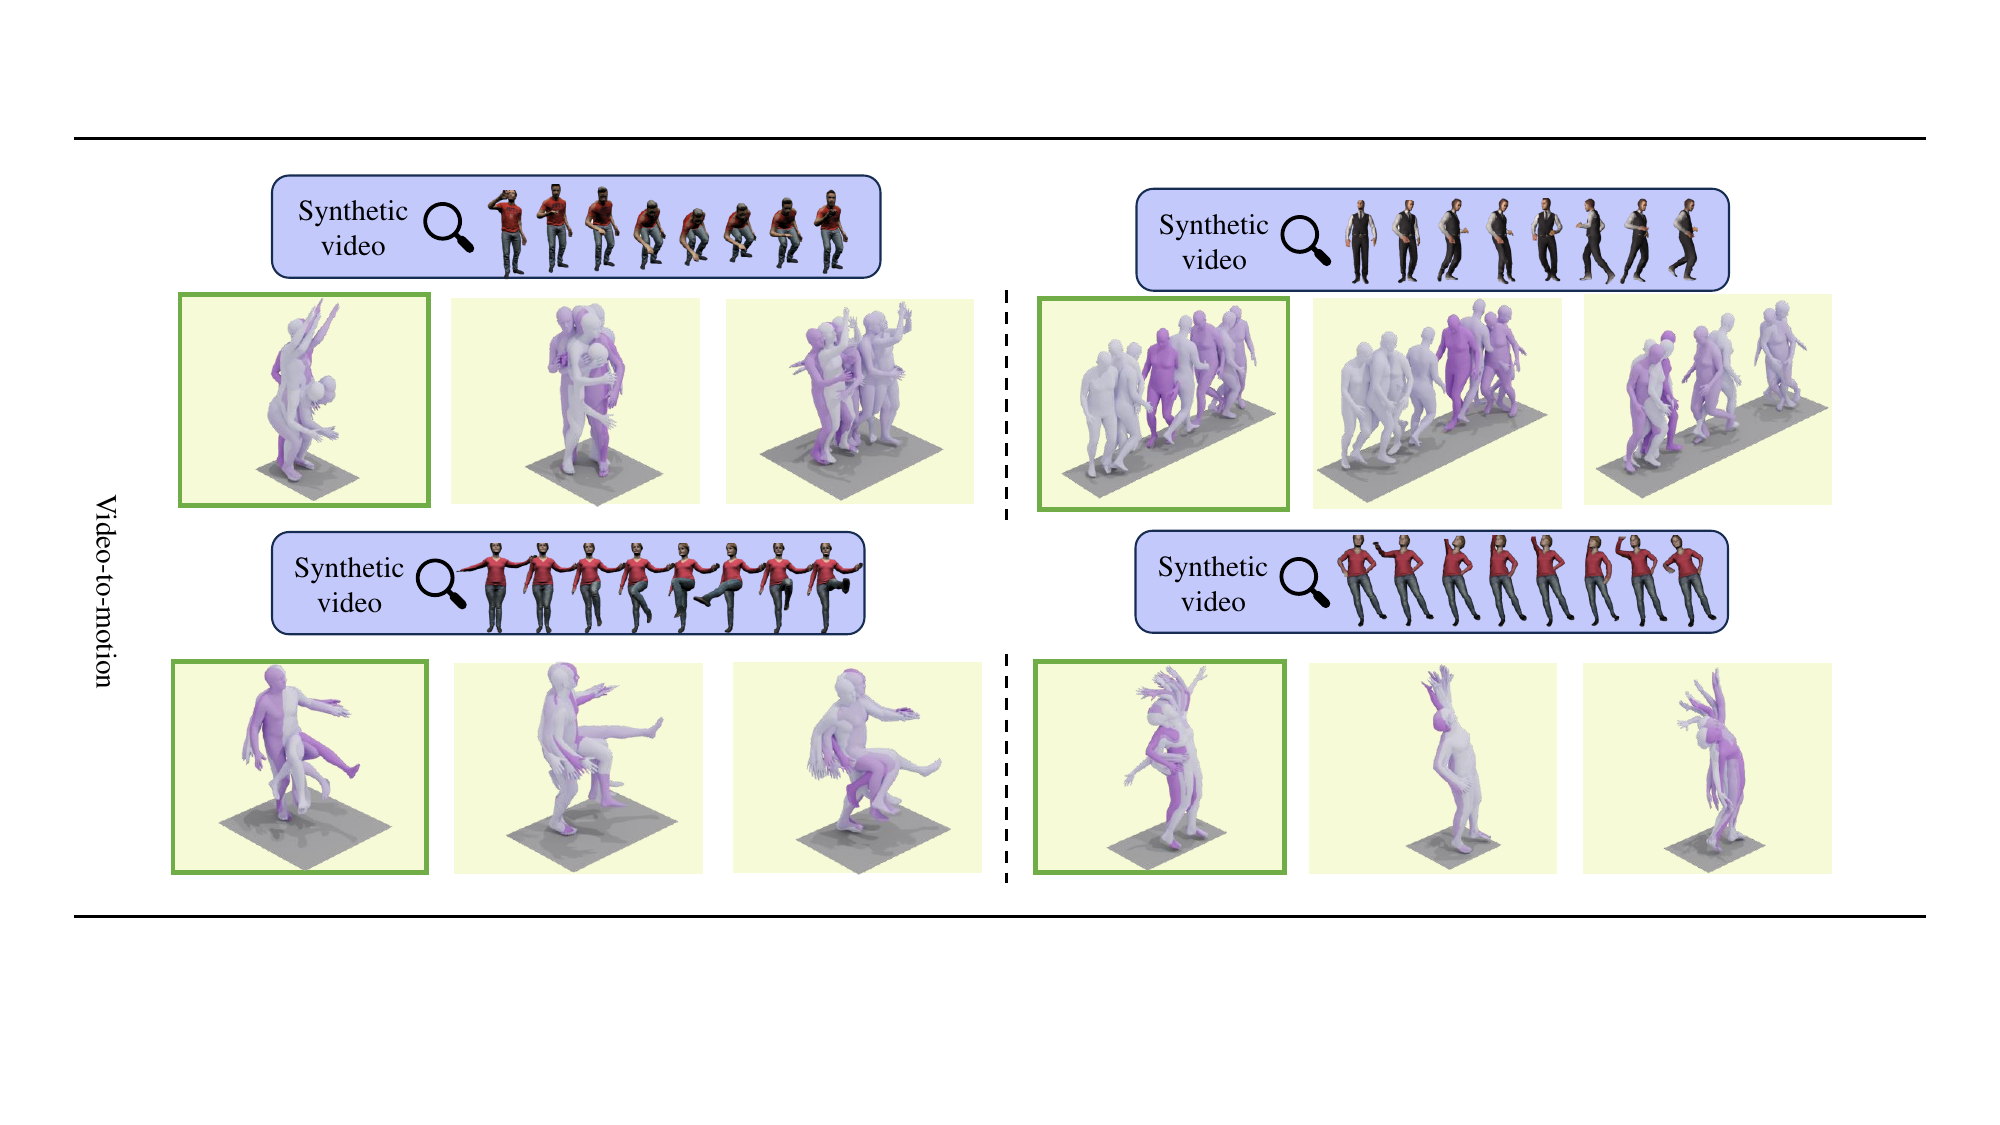}
    \vspace{-1mm}
    \includegraphics[width=\textwidth]{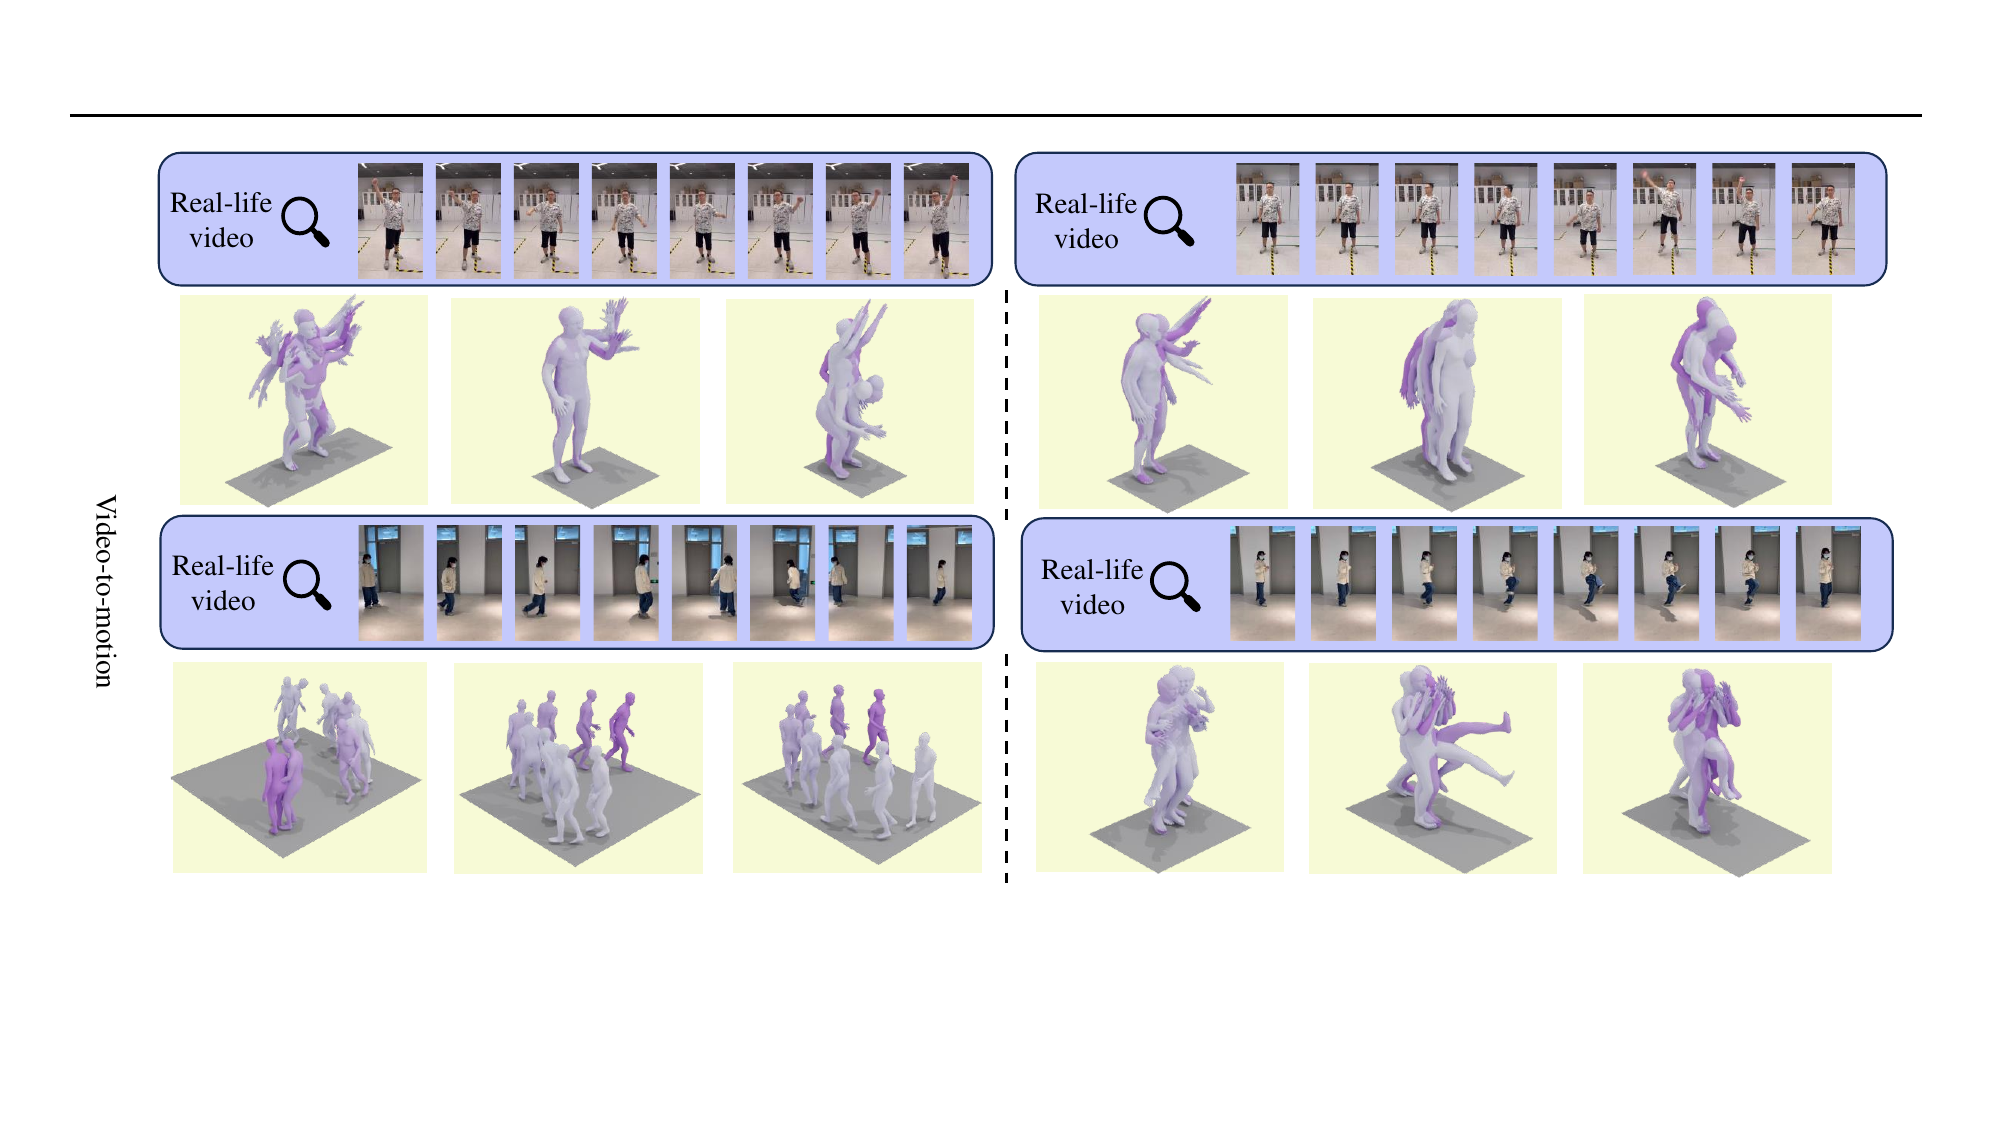}
    \beforefigcaption
    \caption{\textbf{Qualitative Comparison on the HumanML3D Dataset.}}
    \afterfigcaption
    \label{fig:4}
\end{figure*}

% Having the supplementary compiled together with the main paper means that:
% % 
% \begin{itemize}
% \item The supplementary can back-reference sections of the main paper, for example, we can refer to \cref{sec:intro};
% \item The main paper can forward reference sub-sections within the supplementary explicitly (e.g. referring to a particular experiment); 
% \item When submitted to arXiv, the supplementary will already included at the end of the paper.
% \end{itemize}
% % 
% To split the supplementary pages from the main paper, you can use \href{https://support.apple.com/en-ca/guide/preview/prvw11793/mac#:~:text=Delete%20a%20page%20from%20a,or%20choose%20Edit%20%3E%20Delete).}{Preview (on macOS)}, \href{https://www.adobe.com/acrobat/how-to/delete-pages-from-pdf.html#:~:text=Choose%20%E2%80%9CTools%E2%80%9D%20%3E%20%E2%80%9COrganize,or%20pages%20from%20the%20file.}{Adobe Acrobat} (on all OSs), as well as \href{https://superuser.com/questions/517986/is-it-possible-to-delete-some-pages-of-a-pdf-document}{command line tools}.
